# Supplementary material for: Data Selection Curriculum for Neural Machine Translation
Source: arXiv:2203.13867 source file (2022-03-25)
Supplement: Supplementary file 1 [file apn_in_domain_corp.tex]

For high-resource language pairs, we consider {formal} bitext corpora sources as in-domain ($\mathcal{D}_{d} \subset \mathcal{D}_g$), while for low-resource pairs, we do not differentiate between general-domain and in-domain corpus ($\mathcal{D}_{d} \coloneqq \mathcal{D}_g$). 
Table \ref{tab:indomain-corp} presents the in-domain corpora list for high-resource language pairs.

\begin{table}[H]
\centering
\scalebox{0.8}{
\begin{tabular}{l|l}
\toprule
{\textbf{Pair}} & \textbf{In-domain Corpora} \\
\midrule
En-De     & Europarl, News Commentary  \\
En-Hu     & EUconst, Europarl, GlobalVoices, Wikipedia, \\
& WikiMatrix, WMT-News    \\ 
En-Et     &  EUconst, Europarl, WikiMatrix, WMT-News   \\ 
 
\bottomrule
\end{tabular}
}
\caption{In-domain corpora for high-resource language pairs.}
\label{tab:indomain-corp-ap}
\end{table}
