# Supplementary material for: Data Selection Curriculum for Neural Machine Translation
Source: arXiv:2203.13867 source file (2022-03-25)
Supplement: Supplementary file 2 [file apn_res.tex]

Comparing the performance of traditional fine-tuning (\textit{All Data} in Table~\ref{tab:low-res-main-results}) with the \textit{Converged Model }for low-resource languages, we see that both of these perform on par. This is not surprising as both approaches use all the train data ($\mathcal{D}_g$) during the whole training (for low-resource languages $\mathcal{D}_{d} \coloneqq \mathcal{D}_g$). The only difference between the two approaches is ---- while the converged model continues to train the base model from warm-up stage, the traditional fine-tuning approach resets the base model's meta-parameters (e.g., learning-rate, lr-scheduler, dataloader, optimizer) and continue the training. 

For high-resource languages in Table \ref{tab:high-res-main-results}, while we fine-tune the base model only on the in-domain training data ($\mathcal{D}_d \subset \mathcal{D}_g$) in traditional fine-tuning (\textit{All In-domain Data} in the Table), the converged model continues to train the base model on all the general-domain data ($\mathcal{D}_g$). Here, traditional fine-tuning performs better than the converged model on En-De (+0.4) and En-Et (+0.9), while exhibits worse performance on the other four directions by 0.7 BLEU score on an average.
